# Supplementary material for: Sketched Newton-Raphson
Source: arXiv:2006.12120 source file (2022-05-09)
Supplement: Supplementary file 1 [file SNR_siam_appendix.tex]

\section{Additional experimental details and the complexity} \label{sec:detailexp}

%All the sampling of the methods was pre-computed before starting counting the wall-clock time for each method and each dataset. We also paused the timing the performance evaluation of the gradient norm or other measurements such as the logistic regression loss that were necessary to generate the plots.
%In the following, from the experimental results for GLM in Section~$8$ in the main paper, we discuss the parameters' choices for TCS in practice, including the sketching sizes $(\tau_d, \tau_n)$, the Bernoulli parameter $p$, the stepsize $\gamma$ and the analysis of complexity.
See Table~\ref{tab:parameters} for the parameters we chose for TCS in the experiments in Fig.~\ref{figure}. Such choices are due to TCS's cost per iteration which involves the feature dimension $d$, the number of the data samples $n$, the sketch sizes $(\tau_d, \tau_n)$ and the Bernoulli parameter $b$. Here we only consider datasets with $d \ll n$.

It is beneficial to first understand TCS's cost in the simple setting where $\tau_d = \tau_n = 1$. The cost per iteration is stochastic and depends on the nature of the sketch. 

\ruiline{
When performing the updates~\eqref{eq:update} with $(d, \tau_d)$-block sketch, we sketch the first $d$ rows of~\eqref{eq:F}. As $\tau_d = 1$, let $\mS_d = e'_j \in \R^{d\times1}$ with $e'_j$ the $j$th unit coordinate in $\R^d$.
For $\mS_k =
\begin{bmatrix}
\mS_d & 0 \\
0 & 0
\end{bmatrix} $ with $\mS_d = e'_j$ at $k$th iteration, we get
\vspace{-.1in}
\begin{eqnarray}
\alpha^{k+1}_i &=& \alpha^k_i - \gamma \cdot \frac{\frac{\mA_{ji}}{\lambda n}\left(\frac{1}{\lambda n}\left[\mA\alpha^k\right]_j - w_j^k\right)}{\frac{1}{\lambda^2n^2}[\mA\mA^\top]_{jj}+1}, \quad \mbox{for all } i = 1, \cdots, n, \\
w^{k+1}_j &=& w^k_j + \gamma \cdot \frac{\frac{1}{\lambda n}\left[\mA\alpha^k\right]_j - w_j^k}{\frac{1}{\lambda^2n^2}[\mA\mA^\top]_{jj}+1}.
\end{eqnarray}
 The cost of this iteration can be $\cO(n)$ with $n$ coordinates' updates of the auxiliary variable $\alpha$.
% This is affordable as the cost of each coordinate's update is $1$. Besides $\mA$ is often sparse. The update in this case can be much cheaper than $n$. 
Indeed, the term $\frac{1}{\lambda^2n^2}[\mA\mA^\top]_{jj}$ is pre-computed and stored in the fixed matrix $\frac{1}{\lambda^2n^2}\mA\mA^\top\in\R^{d \times d}$. We also introduce an auxiliary variable $\overline{\alpha}^k$ to keep tracking the term $\overline{\alpha}^k = \frac{1}{\lambda n}\mA\alpha^k \in \R^d$. The vector $\overline{\alpha}^k$ can be efficiently updated by
\begin{align}
\overline{\alpha}^{k+1} = \overline{\alpha}^k - \gamma \cdot \frac{\overline{\alpha}^k_j - w_j^k}{\frac{1}{\lambda^2n^2}[\mA\mA^\top]_{jj}+1} \cdot [\mA\mA^\top]_{j}, 
\end{align}
where $[\mA\mA^\top]_{j}$ is the $j$th column of $\mA\mA^\top$. Thus the update of $\overline{\alpha}^k$ costs $\cO(d)$.
Notice that we only update one single coordinate of $w$ from this sketch, i.e.\ $w_j$. 
}

\ruiline{
Alternatively, when performing the updates~\eqref{eq:update} with $(n, \tau_n)$-block sketch, we sketch the last $n$ rows of~\eqref{eq:F}. For $\mS_k =
\begin{bmatrix}
0 & 0 \\
0 & \mS_n
\end{bmatrix} $ with $\mS_n = e_i$ the $i$th unit coordinate in $\R^n$ at $k$th iteration, we get
\vspace{-.1in}
\begin{align}
\alpha^{k+1}_i &= \alpha^k_i - \gamma \cdot \frac{\alpha_i^k + \phi_i'(a_i^\top w^k)}{\|a_i\|_2^2\phi_i''(a_i^\top w^k)^2 + 1}, \\
w^{k+1} &= w^k - \gamma \cdot \frac{\alpha_i^k + \phi_i'(a_i^\top w^k)}{\|a_i\|_2^2\phi_i''(a_i^\top w^k)^2 + 1} \cdot \phi_i''(a_i^\top w^k)a_i, \\
\overline{\alpha}^{k+1} &= \overline{\alpha}^k - \gamma \cdot \frac{\alpha_i^k + \phi_i'(a_i^\top w^k)}{\|a_i\|_2^2\phi_i''(a_i^\top w^k)^2 + 1} \cdot \frac{1}{\lambda n} a_i.
\end{align}
The cost of this iteration is $\cO(d)$ with the full coordinates' updates of $w, \overline{\alpha}$ and a single coordinate update of $\alpha$. If we choose $b = n/(n+d)$ to sample one row of~\eqref{eq:F} uniformly, the cost per iteration in expectation will be
\begin{align}
\mbox{Cost(update TCS)} = \cO(n) * (1-b) + \cO(d) * b = \cO(nd/(n+d)) = \cO(\min(n,d)).
\end{align}}
\vspace{-.2in}

Consequently, the TCS method in average has the same cost as \SGD, i.e.\ $\cO(d)$ in the case $d \ll n$. Increasing $\tau_d$ and $\tau_n$ drops significantly the number of iterations, but increases the total cost per iteration. 
%For instance, the total cost can be $\cO(\tau_n^2 d)$ with $\tau_n = 50, 150$ (e.g.\ \emph{covtype, a9a, webspam, phishing}) or $\cO(\tau_n^3)$ with $\tau_n = 50, 150 > d$ (e.g.\ \emph{fourclass, artificial, ijcnn1}) according to different cases. 
Thus there is a trade off between increasing the sketch sizes and keeping the total cost per iteration low.
For the total cost in general with different choices of $\tau_d, \tau_n$ and $b$, please refer it on arXiv\footnote{Section H: Complexity analysis for TCS in different cases \url{https://arxiv.org/pdf/2006.12120.pdf}.} for more details.

Different to our global convergence theories, in practice, choosing constant stepsize $\gamma > 1$ may converge faster for certain datasets. Here we need to be careful that the stepsize we mentioned is the stepsize used for $(n, \tau_n)$-block sketch. As for $(d, \tau_d)$-block sketch, we always choose $\gamma = 1$, which solves exactly the linear system.
%Henceforth, we use $\gamma$ to designate the stepsize used for the sketch of the last $n$ rows of~\eqref{eq:F}.
In our experiments, we found that the choice of the stepsize is related to C.N.\ of the model.
% which is already discussed in Section~\ref{sec:experiments}.
If the dataset is ill-conditioned with a big C.N., $\gamma = 1$ is a good choice (Fig.~\ref{figure} top row except for a9a); if the dataset is well-conditioned with a small C.N., all $\gamma \in (1, 1.8]$ still converges. In practice, $\gamma = 1.8$ is a good choice for well-conditioned datasets (Fig.~\ref{figure} bottom row). For a9a, we did a grid search for the stepsize.
%However, from the grid search of stepsizes for a9a, we know that the optimal stepsize for a9a is $\gamma = 1.5$.
%Also from Figure~\ref{fig:a9a} with stepsize $\gamma = 1.5$, $p = p_{uniform} - 0.03$ obtained by the selection rule of $p$ is showed as a good choice.
To avoid tuning the stepsizes, it is possible to apply a stochastic line search process~\cite{Stochastic_Line_Search_nips2019} in our method TCS without increasing its complexity. Please refer it on arXiv\footnote{Section I \url{https://arxiv.org/pdf/2006.12120.pdf}.} for more details.
% because of the page constraint.

\begin{table}
  \caption{Details of the parameters' choices ($\gamma$ and $b$) for $50$-TCS, $150$-TCS and $300$-TCS}
  \label{tab:parameters}
  \centering
  \begin{tabular}{ ccccc }
     \toprule
                 &            & $50$-TCS                        & $150$-TCS                      & $300$-TCS             \\
     \cmidrule(r){3-5}
     dataset     & stepsize   & Bernoulli              & Bernoulli             & Bernoulli    \\
     \midrule
     covetype    & $1.0$      & $\frac{n}{n + \tau_n * 3}$      & $\frac{n}{n + \tau_n * 3}$     & $\frac{n}{n + \tau_n * 3}$       \\
     a9a         & $1.5$      & $\frac{n}{n + \tau_n} - 0.03$   & $\frac{n}{n + \tau_n} - 0.03$  & $\frac{n}{n + \tau_n} - 0.11$    \\
     fourclass   & $1.0$      & $\frac{n}{n + \tau_n} - 0.11$   & $\frac{n}{n + \tau_n} - 0.11$  & $\frac{n}{n + \tau_n} - 0.11$    \\
     artificial  & $1.0$      & $\frac{n}{n + \tau_n} - 0.03$   & $\frac{n}{n + \tau_n} - 0.11$  & $\frac{n}{n + \tau_n} - 0.11$    \\
     ijcnn1      & $1.8$      & $\frac{n}{n + \tau_n} - 0.03$   & $\frac{n}{n + \tau_n} - 0.11$  & $\frac{n}{n + \tau_n} - 0.11$    \\
     webspam     & $1.8$      & $\frac{n}{n + \tau_n * 3}$      & $\frac{n}{n + \tau_n * 3}$     & $\frac{n}{n + \tau_n * 3}$       \\
     epsilon     & $1.8$      & $\frac{n}{n + \tau_n * 3}$      & $\frac{n}{n + \tau_n * 3}$     & $\frac{n}{n + \tau_n * 3}$       \\
     phishing    & $1.8$      & $\frac{n}{n + \tau_n} - 0.03$   & $\frac{n}{n + \tau_n} - 0.11$  & $\frac{n}{n + \tau_n} - 0.11$    \\
     \bottomrule
  \end{tabular}
\end{table}
